# Supplementary material for: CoBERL: Contrastive BERT for Reinforcement Learning
Source: arXiv:2107.05431 source file (2022-02-22)
Supplement: Supplementary file 1 [file further_discussion.tex]

\section{Additional discussion}
\label{app:extra-discussion}

The architecture of \agent{} is based on the idea of combining two forms of memory (an LSTM and a Tranformer stack) to combine the benefits of each of these.
In particular, the LSTM is known for having a short contextual memory. However, by putting a transformer before the LSTM, the embeddings provided to the LSTM have already benefited from the ability of the Transformer stack to process long contextual dependencies, thus helping the LSTM in this respect. The second benefit works in a complementary direction. One problem with Transformer is that the computational complexity is quadratic with respect to the sequence length. So running a Transformer with large contextual memory is very expensive. Our idea is that by letting an LSTM process some of this contextual information we can reduce the memory size of the Transformer up to the point where we see a loss in performance. 
The first hypothesis was empirically confirmed by the ablation in Table \ref{tab:ablation_num_params} where we put the LSTM before the Transformer. However, this proved to be useless as the Transformer does not need extra context on the inputs side given its ability to process long term dependencies.  This combined with the shorter transformer memory size of \agent{} resulted in much worse performance.
The second hypothesis was empirically confirmed by the ablation in Table \ref{tab:ablation_architecture_results} where we remove the LSTM. In this case, given that \agent{} was run with a shorter memory size than \cite{parisotto2020stabilizing} it performed much worse.
This ablation resulted in worse performance (here the memory size of Transformer was the same as in \agent{}).

In terms of skip connections, the one between the GTrXL module and the LSTM, was done to give the ability to \agent{} to initially skip the output of the Transformer stack until the weights of this were warmed-up. That is also the reason why we implemented a learnt gate. The idea is that, once the transformer starts to output useful information then the agent will be able to tune the weights in the gate to learn from them. We figured this would also help in terms of data efficiency as at the beginning of training the agent could quickly use the LSTM to get off the ground to start collecting interesting data. \agent{} is indeed better in data efficiency as shown by Table \ref{tab:atari_results} (5th and 25th percentile), Figure \ref{fig:dm_lab_plots}B, and Appendix \ref{app:learning-curves}.
